# Supplementary material for: Surface defects, flavored modular differential equations and modularity
Source: arXiv:2207.10463 source file (2022-08-03)
Supplement: Supplementary file 1 [file monodromy.tex]

%!TEX root = ../defectIndexAndMDE.tex

\section{Monodromy}\label{app:monodromy}

\subsection{\texorpdfstring{$\mathfrak{so}(8)_{-2}$}{}}

We can solve the equation (\ref{unflavored-MDE-I04}) by rewriting it in terms of $\lambda\left(\tau\right)=\frac{\vartheta_2(\tau)^4}{\vartheta_3(\tau)^4}$, and transform it into an ODE as follows:
\begin{align}
\frac{1}{4}\left(\lambda-1\right)^2D^2_{\lambda}\chi\left(\lambda\right)+\frac{1}{12}\left(\lambda^2-1\right)D_{\lambda}\chi(\lambda)-\frac{35}{144}\left(\lambda^2-\lambda+1\right)\chi(\lambda)=0
\end{align}
Let $\chi\left(\lambda\right)=\left(1-\lambda\right)^{-5/6}\phi(\lambda)$, then function $\phi\left(\lambda\right)$ is solution of the following generalized hypergeometric equations:
\begin{align}
\left(D_{\lambda}-\beta_1\right)\left(D_{\lambda}-\beta_2\right)\phi\left(\lambda\right)-\lambda\left(D_{\lambda}+1-\alpha_1\right)\left(D_\lambda+1-\alpha_2\right)\phi(\lambda)=0
\end{align}
the parameters are $\alpha_1=\frac{2}{3}$, $\alpha_2=\frac{8}{3}$, $\beta_1=\frac{7}{6}$, $\beta_2=-\frac{5}{6}$. There are two linear independent solutions for this GHE:
\begin{align}
&\phi_0\left(\lambda\right)=\lambda^{\frac{7}{6}}{}_2F_1\left(\frac{3}{2},-\frac{1}{2};3;\lambda\right)\\
&\phi_1\left(\lambda\right)=G^{2,0}_{2,2}\left(\lambda\right|\left.\begin{array}{cc}
	\frac{2}{3} & \frac{8}{3} \\
	\frac{7}{6} & -\frac{5}{6}
\end{array}\right)
\end{align}
From the integral representation:
\begin{align}
{}_2F_1\left(\frac{3}{2},-\frac{1}{2};3;\lambda\right)=\frac{\Gamma\left(3\right)}{\Gamma\left(\frac{3}{2}\right)\Gamma\left(-\frac{1}{2}\right)}\frac{1}{2\pi i}\int_L\frac{\Gamma\left(\frac{3}{2}+s\right)\Gamma\left(-\frac{1}{2}+s\right)}{\Gamma\left(3+s\right)}\Gamma\left(-s\right)\left(-\lambda\right)^s ds
\end{align}
The integrated function has the following two sets of poles:$s=\frac{1}{2}$, $s=-\frac{1}{2}$, $s=-\frac{3}{2}$, $s=-\frac{5}{2}$ .... and $s=0$, $s=1$, $s=2$.... The former set of poles are arranged at the left hand side of contour $L$, the latter is on the right hand side. To obtain its Taylor expansion within $|\lambda|<1$, we pick up the residues of the poles at the right hand side of $L$, and have:
\begin{align}
{}_2F_1\left(\frac{3}{2},-\frac{1}{2};3;\lambda\right)=-\frac{2}{\pi}\sum_{n\geq 0}\frac{\Gamma\left(\frac{3}{2}+n\right)\Gamma\left(n-\frac{1}{2}\right)}{n!\Gamma\left(n+3\right)}\lambda^n\qquad |\lambda|<1
\end{align}
To obtain its Laurent expansion when $|\lambda|>1$, we simply pick up the residues of poles at the left hand side of contour $L$:
\begin{align}
&{}_2 F_1\left(\frac{3}{2},-\frac{1}{2};3;\lambda\right)=\frac{32}{15\pi}\left(-\lambda\right)^{\frac{1}{2}}+\frac{8}{3\pi}\left(-\lambda\right)^{-\frac{1}{2}}-\frac{2}{\pi}\sum_{n\geq 0}\frac{(-)^{n+1}}{\pi}\frac{\left(-\lambda\right)^{-\frac{3}{2}-n}\Gamma\left(\frac{3}{2}+n\right)\Gamma\left(n-\frac{1}{2}\right)}{n!\Gamma\left(n+3\right)}\notag\\
&\left(A_n+A_{n+2}-\psi\left(\frac{3}{2}+n\right)-\psi\left(\frac{3}{2}-n\right)+\ln\left(-\lambda\right)\right)\qquad |\lambda|>1
\end{align}
If we set $\left(-\right)=e^{\pi i}$, $\ln(-\lambda)=\ln\lambda+\pi i$, we have:
\begin{align}
&{}_2 F_1\left(\frac{3}{2},-\frac{1}{2};3;\lambda\right)=\frac{32 i}{15\pi}\left(\lambda\right)^{\frac{1}{2}}-\frac{8 i}{3\pi}\left(\lambda\right)^{-\frac{1}{2}}+\frac{2 i}{\pi^2}\sum_{n\geq 0}\frac{\Gamma\left(\frac{3}{2}+n\right)\Gamma\left(n-\frac{1}{2}\right)}{n!\Gamma\left(n+3\right)}\lambda^{-\frac{3}{2}-n}\notag\\
&\left(A_n+A_{n+2}-\psi\left(\frac{3}{2}+n\right)-\psi\left(\frac{3}{2}-n\right)+\ln\left(\lambda\right)+\pi i\right)\qquad |\lambda|>1
\end{align}
And the Meijers G function have the following integral representation( some basic property about Meijer's G function are included in \cite{BeukerMeijersG}):
\begin{align}
G^{2,0}_{2,2}\left(\lambda\right|\left.\begin{array}{cc}
	\frac{2}{3} & \frac{8}{3} \\
	\frac{7}{6} & -\frac{5}{6}
\end{array}\right)=\frac{1}{2\pi i}\int_L \frac{\Gamma\left(\frac{7}{6}+s\right)\Gamma\left(-\frac{5}{6}+s\right)}{\Gamma\left(\frac{2}{3}+s\right)\Gamma\left(\frac{8}{3}+s\right)}\lambda^{-s}ds
\end{align}
The poles are $s=\frac{5}{6}$, $s=\frac{-1}{6}$, $s=\frac{-7}{6}$,... on th left of contour $L$, pick up all the residues at these poles we have the following Taylor series within $|\lambda|<1$:
\begin{align}
&G^{2,0}_{2,2}\left(\lambda\right|\left.\begin{array}{cc}
	\frac{2}{3} & \frac{8}{3} \\
	\frac{7}{6} & -\frac{5}{6}
\end{array}\right)=\frac{16}{15\pi}\lambda^{-\frac{5}{6}}-\frac{4}{3\pi}\lambda^{\frac{1}{6}}+\frac{1}{\pi^2}\sum_{n\geq 0}\lambda^{\frac{7}{6}+n}\frac{\Gamma\left(n-\frac{1}{2}\right)\Gamma\left(\frac{3}{2}+n\right)}{n!\Gamma\left(n+3\right)}\left(A_n+A_{n+2}-\psi\left(\frac{3}{2}+n\right)\right.\notag\\
&\left.-\psi\left(\frac{3}{2}-n\right)-\ln\lambda\right)\qquad |\lambda|<1
\end{align}
And the integral representation will tell you that when $|\lambda|>1$, $G^{2,0}_{2,2}\left(\lambda\right|\left.\begin{array}{cc}
	\frac{2}{3} & \frac{8}{3} \\
	\frac{7}{6} & -\frac{5}{6}
\end{array}\right)=0$, but we can properly set:
\begin{align}\label{Gextension04}
	G^{2,0}_{2,2}\left(\lambda\right|\left.\begin{array}{cc}
		\frac{2}{3} & \frac{8}{3} \\
		\frac{7}{6} & -\frac{5}{6}
	\end{array}\right)=\lambda^{\frac{5}{6}} G^{2,0}_{2,2}\left(\frac{1}{\lambda}\right|\left.\begin{array}{cc}
	\frac{2}{3} & \frac{8}{3} \\
	\frac{7}{6} & -\frac{5}{6}
\end{array}\right)\qquad |\lambda|>1
\end{align}
For later covenience we normalize the solutions as:
\begin{align}
&\chi_0\left(\lambda\right)=\frac{1}{16\times 2^{\frac{2}{3}}}\left(1-\lambda\right)^{-\frac{5}{6}}\lambda^{\frac{7}{6}}{}_2F_1\left(\frac{3}{2},-\frac{1}{2};3;\lambda\right)
&\chi_{1}\left(\lambda\right)=\frac{1}{8\times 2^{\frac{2}{3}}}\left(1-\lambda\right)^{-\frac{5}{6}}G^{2,0}_{2,2}\left(\lambda\right|\left.\begin{array}{cc}
	\frac{2}{3} & \frac{8}{3} \\
	\frac{7}{6} & -\frac{5}{6}
\end{array}\right)
\end{align}
It is obvious that (when $|\lambda|<1$):
\begin{align}
\chi_0\left(e^{2\pi i}\lambda\right)=e^{\frac{7\pi i}{3}}\chi_0\left(\lambda\right)
\end{align}
By using the series expansion within $|\lambda|<1$, we can readily obtain:
\begin{align}
	\chi_1\left(e^{2\pi i}\lambda\right)=e^{\frac{\pi i}{3}}\chi_1\left(\lambda\right)+2i e^{\frac{\pi i}{3}}\chi_0\left(\lambda\right)
\end{align}
Therefore we have the monodromy around $0$:
\begin{align}
M_0=T^2=\left(\begin{array}{cc}
	e^{\frac{7\pi i}{3}} & o \\
	2e^{\frac{5\pi i}{6}} & e^{\frac{\pi i}{3}}
\end{array}\right)
\end{align}
About the $STS$ transformation, knowing ${}_2F_1\left(\frac{3}{2},\frac{-1}{2};3;\lambda\right)$'s behaviour when $|\lambda|<1$, we have:
\begin{align}
&\chi_0\left(\frac{1}{\lambda}\right)=\frac{1}{16\times 2^{2/3}}\left(1-\frac{1}{\lambda}\right)^{-\frac{5}{6}}\lambda^{-\frac{7}{6}}{}_2F_1\left(\frac{3}{2},\frac{-1}{2};3;1/\lambda\right)\notag\\
&=\frac{e^{\frac{-5\pi i}{6}}}{16\times 2^{2/3}}\left(1-\lambda\right)^{-\frac{5}{6}}\lambda^{-\frac{1}{3}}\left(2i\lambda^{\frac{1}{3}}G^{2,0}_{2,2}\left(\frac{1}{\lambda}\right|\left.\begin{array}{cc}
	\frac{2}{3} & \frac{8}{3} \\
	\frac{7}{6} & -\frac{5}{6}
\end{array}\right)+\lambda^{\frac{3}{2}}{}_2F_1\left(\frac{3}{2},-\frac{1}{2};3;\lambda\right)\right)\notag\\
&=e^{\frac{-\pi i}{3}}\chi_1\left(\lambda\right)+e^{-\frac{5\pi i}{6}}\chi_0\left(\lambda\right)\qquad |\lambda|<1
\end{align}
From the extension we choose \ref{Gextension04} we also have:
\begin{align}
\chi_1\left(\frac{1}{\lambda}\right)=-e^{\frac{\pi i}{6}}\chi_1\left(\lambda\right)\qquad |\lambda|<1
\end{align}
Therefore under $STS$ transformation we have:
\begin{align}
M_R=\left(\begin{array}{cc}
	-e^{\frac{\pi i}{6}}& -e^{\frac{2\pi i}{3}}\\
	0 & -e^{\frac{\pi i}{6}}
\end{array}\right)
\end{align}

\subsection{$\mathcal{N} = 4$}

In terms of $\Gamma(2)$ haupt function $\lambda(\tau)=\frac{\vartheta_2(\tau)^4}{\vartheta_3(\tau)^4}$, twisted LMDE \ref{MDE-weight-two-unflavored-N4} can be expressed as the following generalized hypergeometric equation\cite{Naculich:1989NuPhB.323..423N}:
\begin{align}
\left(D-\beta_1\right)\left(D-\beta_2\right)\chi(\lambda(\tau))-\lambda\left(D+1-\alpha_1\right)\left(D+1-\alpha_2\right)\chi(\lambda(\tau))=0
\end{align}
where $\alpha_1=\frac{1}{4}$, $\alpha_2=\frac{5}{4}$, $\beta_1=\frac{3}{4}$, $\beta_2=-\frac{1}{4}$, $D$ represents $\lambda\frac{d}{d\lambda}$. This equation admits the following two solutions near $\lambda=0$:
\begin{align}
&\chi_0(\lambda)=\frac{1}{8}\lambda^{3/4}\,{}_2F_1\left(\frac{3}{2},\frac{1}{2};2;\lambda\right)\\
&\chi_1(\lambda)=\pi G_{2,\,2}^{2,\,0} \left( {\begin{matrix}    {} & {1/4,5/4}  \cr    {- 1/4, 3/4\,} & {}  \cr  \end{matrix} \;\left| {\;\lambda} \right.} \right)=\frac{\pi}{2\pi i}\int_L\frac{\Gamma\left(s-\frac{1}{4}\right)\Gamma\left(\frac{3}{4}+s\right)}{\Gamma\left(s+\frac{1}{4}\right)\Gamma\left(\frac{5}{4}+s\right)}\lambda^{-s}ds
\end{align}
with $L$ as a contour at the right side of a sequence of poles $s=\frac{1}{4}$, $s=-\frac{3}{4}$, ..., $s=-n+\frac{1}{4}$.
\begin{tikzpicture}
\fill (0.25cm,0) circle (2pt) node[below]{\tiny $\frac{1}{4}$};
\fill (-0.75cm,0) circle (2pt) node[below]{\tiny $-\frac{3}{4}$};
\fill (-1.75cm,0) circle (2pt) node[below]{\tiny $-\frac{7}{4}$};
\fill (-2.75cm,0) circle (2pt) node[below]{\tiny $-\frac{11}{4}$};
\draw [->](-3cm,0)--(3cm,0);
\draw [->](0,-2cm)--(0,2cm);
\draw [red,thick,->](0.5cm,-2cm)--(0.5cm,2cm) 
node[near start]{$L$};
\end{tikzpicture}

 We can easily get series expression of $\chi_1$ converging within the unit disk $0<|\lambda|<1$ by picking up the residues mentioned previously:
\begin{align}
&\chi_1(\lambda)=\frac{2}{\lambda^{1/4}}+\frac{\lambda^{3/4}}{\pi}\sum_{n=0}^{\infty}\frac{\Gamma\left(\frac{3}{2}+n\right)\Gamma\left(\frac{1}{2}+n\right)}{n!\Gamma\left(n+2\right)}\left(-\psi\left(-n-\frac{1}{2}\right)-\psi\left(\frac{1}{2}-n\right)-\ln \lambda+A_n+A_{n+1}\right)\lambda^{n}\notag\\
&=\frac{2}{\lambda^{1/4}}-4\ln \lambda \chi_0(\lambda)-\frac{1}{2}\sum_{n=0}^{\infty}\frac{\left(\frac{3}{2}\right)_n\left(\frac{1}{2}\right)_n}{n!\left(2\right)_n}\left(\psi\left(-n-\frac{1}{2}\right)+\psi\left(\frac{1}{2}-n\right)-A_n-A_{n+1}\right)\lambda^{n+3/4} 
\end{align}
where $A_n$ is the following:
\begin{align}
A_n=-\gamma+\frac{1}{1}+\frac{1}{2}+\frac{1}{3}+...+\frac{1}{n}
\end{align}
It is worth noting that:
\begin{align}
	& G_{2,\,2}^{2,\,0} \left( {\begin{matrix}
			{} & {a,a + 1}  \cr    {a - 1/2,a + 1/2\,} & {}  \cr  \end{matrix} \;\left| {\;z} \right.} \right) =   \cr 
	&  = {2 \over \pi }\theta \left( {1 - \left| z \right|} \right)z^{a - {1 \over 2}} E\left( {1 - z} \right)
	\quad \left| {\;z \notin \left( { - 1,0} \right)} \right.
\end{align}
which means that within the unit disk $\chi_1(\lambda)=2\lambda^{-\frac{1}{4}}E(1-\lambda)$ when $\lambda\notin \left(-1,0\right)$. $E$ represents the Elliptic E function. It is natural that monodromy matrix around $0$ is:
\begin{align}
M_0=\left(
\begin{matrix}
	&-i   &0\\
	&8\pi &-i
\end{matrix}
\right)
\end{align}
Using another base:
\begin{align}
\left(\begin{array}{c}
	\operatorname{ch}_0\\
	\operatorname{ch}_1
\end{array}\right)=\left(\begin{array}{cc}
1 & 0\\                                                          
1 & \frac{1}{4\pi i}
\end{array}\right)\left(\begin{array}{c}
\chi_0\\
\chi_1
\end{array}\right)
\end{align}
we can obtain $T^2$ matrix under bases $\operatorname{ch}_0$ and $\operatorname{ch}_1$:
\begin{align}
M_0^{\prime}=T^2=\left(
\begin{array}{cc}
	-i & 0\\
	-2i & -i\\
\end{array}\right)
\end{align}
We can also compute the STS transformation matrix. Observing that acting STS on $\tau$ is equivalent to transforming $\lambda$ to $\frac{1}{\lambda}$, we believe that $\chi_0\left(\frac{1}{\lambda}\right)$ and $\chi_{1}\left(\frac{1}{\lambda}\right)$ are also solutions to this hypergeometric equation. Therefore they should be linear combinations of $\chi_0(\lambda)$ and $\chi_1(\lambda)$. We can determine the coefficient of linear combinations by looking at $\chi_0\left(\frac{1}{\lambda}\right)$ and $\chi_1\left(\frac{1}{\lambda}\right)$'s behaviours near $\lambda=0$ and $\lambda=\infty$. For $\chi_0\left(\frac{1}{\lambda}\right)$, if we want to determine its behaviour around $\lambda=0$, we need to know the analytic continuation to $\infty$ of $\chi_0\left(\lambda\right)$. In fact, for ${}_{2}F_{1}\left(\frac{3}{2},\frac{1}{2};2,\lambda\right)$, it has the following integral representation:
\begin{align}
{}_2 F_1\left(\frac{3}{2},\frac{1}{2};2,\lambda\right)=\frac{\Gamma\left(2\right)}{\Gamma\left(\frac{3}{2}\right)\Gamma\left(\frac{1}{2}\right)}\frac{1}{2\pi i}\int_L \frac{\Gamma\left(s+\frac{3}{2}\right)\Gamma\left(s+\frac{1}{2}\right)\Gamma\left(-s\right)}{\Gamma\left(s+2\right)}\left(-\lambda\right)^s ds
\end{align}
The contour $L$ is depicted as follows:
\begin{tikzpicture}
	\fill (-0.5cm,0) circle (2pt) node[below]{\tiny $-\frac{1}{2}$};
	\fill (-1.5cm,0) circle (2pt) node[below]{\tiny $-\frac{3}{2}$};
	\fill (-2.5cm,0) circle (2pt) node[below]{\tiny $-\frac{5}{2}$};
	\fill (0,0) circle (2pt) node[below]{\tiny $0$};
		\fill (1cm,0) circle (2pt) node[below]{\tiny $1$};
		\fill (2cm,0) circle (2pt) node[below]{\tiny $2$};
	\draw [->](-3cm,0)--(3cm,0);
	\draw [->](0,-2cm)--(0,2cm);
	\draw [red,thick,->](-0.25cm,-2cm)--(-0.25cm,2cm) 
	node[near start]{$L$};
\end{tikzpicture}
To study the behaviour when $|\lambda|<1$, we simply pick up the residues of the poles on the right hand side:
\begin{align}
&{}_2 F_1\left(\frac{3}{2},\frac{1}{2};2,\lambda\right)=\frac{\Gamma\left(2\right)}{\Gamma\left(\frac{3}{2}\right)\Gamma\left(\frac{1}{2}\right)}\sum_{n\geq 0}\operatorname{Res}_{s=n}\left(\frac{\Gamma\left(s+\frac{3}{2}\right)\Gamma\left(s+\frac{1}{2}\right)\Gamma\left(-s\right)}{\Gamma\left(s+2\right)}\left(-\lambda\right)^s\right)\\
&=\frac{\Gamma\left(2\right)}{\Gamma\left(\frac{3}{2}\right)\Gamma\left(\frac{1}{2}\right)}\sum_{n\geq 0}\frac{\left(-\right)^n}{n!}\frac{\Gamma\left(n+\frac{3}{2}\right)\Gamma\left(n+\frac{1}{2}\right)}{\Gamma\left(n+2\right)}\left(-\lambda\right)^n=\sum_{n\geq 0}\frac{\left(\frac{3}{2}\right)_n\left(\frac{1}{2}\right)_n}{n!\left(2\right)_n}\lambda^n\qquad \left|\lambda\right|<1
\end{align}
For $\left|\lambda\right|>1$, we can study its Laurent expansion by picking up the residues on the left hand side of the contour $L$:
\begin{align}
&{}_2 F_1\left(\frac{3}{2},\frac{1}{2};2;\lambda\right)=\frac{2}{\pi}\sum_{n\geq 0}\operatorname{Res}_{s=-n-\frac{1}{2}}\left(\frac{\Gamma\left(s+\frac{3}{2}\right)\Gamma\left(s+\frac{1}{2}\right)\Gamma\left(-s\right)}{\Gamma\left(s+2\right)}\left(-\lambda\right)^s\right)\notag\\
&=\frac{2}{\pi}\sum_{n\geq 0}\frac{\left(-\right)^{n+1}\Gamma\left(n+\frac{3}{2}\right)\Gamma\left(n+\frac{1}{2}\right)}{\pi n! \left(n+1\right)!}\left(-\lambda\right)^{-n-\frac{3}{2}}\left(-\psi\left(n+\frac{3}{2}\right)-\psi\left(-n+\frac{1}{2}\right)+\ln\left(-\lambda\right)+A_n+A_{n+1}\right)\notag\\
&+\frac{4}{\pi}\left(-\lambda\right)^{-\frac{1}{2}}\qquad \left|\lambda\right|>1
\end{align}
Take $(-)^{-\frac{1}{2}}=-i$, and $\ln\left(-\lambda\right)=\ln\lambda+\pi i$, and note that $\psi\left(-n-\frac{1}{2}\right)=\psi\left(n+\frac{3}{2}\right)$. Then for $\left|\lambda\right|<1$, we have:
\begin{align}
\chi_0\left(\frac{1}{\lambda}\right)=\frac{-i}{4\pi}\chi_1\left(\lambda\right)+\chi_0\left(\lambda\right)\qquad \left|\lambda\right|<1
\end{align}
And we also have:
\begin{align}
\chi_1\left(\frac{1}{\lambda}\right)=\chi_1\left(\lambda\right)(???)
\end{align}
Therefore we can obtain:
\begin{align}
M_R=\left(\begin{array}{cc}
	1 & \frac{-i}{4\pi} \\
	0 & 1\\
\end{array}\right)
\end{align}
In the $\operatorname{ch}_0\left(\lambda\right)$ and $\operatorname{ch}_1\left(\lambda\right)$ bases, it can be recasted as:
\begin{align}
M_R^{\prime}=\left(\begin{array}{cc}
	0 & 1 \\
	-1 & 2\\
\end{array}\right)
\end{align}

\subsection{$\mathcal{T}_{1,2}$}
The $\mathcal{T}_{1,2}$ in the unflavored limit actually obeys a six order untwisted modular differential equation:
\begin{align}
\left(D_q^{(3)}-220 E_4D_q^{(1)}+700 E_6\right)\mathcal{I}_{1,2}=0
\end{align}
Rewrite the equation in terms of the reciprocal of Klein-J invariant $K(q)=\frac{1}{j(q)}$, we can recast this equation as the following:
\begin{align}
\left(\prod_{i=1}^{3}\left(D_K+\beta_i-1\right)-K\prod_{i=1}^{3}\left(D_K+\alpha_i\right)\right)\chi(K)=0	
\end{align} 
Where $\alpha=0,\frac{1}{3},\frac{2}{3}$, $\beta=\frac{1}{6}, \frac{7}{6}, \frac{7}{6}$, and $D_K$ represents $K\frac{d}{dK}$. We choose to compute the S and T matrix under the following bases, which comes from the $\mathcal{T}_{1,2}$ Schur index and its modular transformation partners:
$$\operatorname{ch}_0\qquad \operatorname{ch}_{\log,1}\qquad \operatorname{ch}_{\log,2}$$
They can be expressed as a linear combinations of the three linear independent series below:
\begin{align}
&\chi_0(K)=K^{5/6}{}_3 F_2\left(\frac{5}{6}, \frac{7}{6}, \frac{3}{2}; K\right)\\
&\chi_1(K)=\frac{-12\pi^{3/2}}{K^{1/6}}+\sum_{n=0}^{\infty}K^{5/6+n}\frac{\Gamma\left(\frac{5}{6}+n\right)\Gamma\left(\frac{7}{6}+n\right)\Gamma\left(\frac{3}{2}+n\right)}{n!\left(n+2\right)!\left(n+2\right)!}\left(\psi\left(\frac{5}{6}+n\right)+\psi\left(\frac{7}{6}+n\right)+\psi\left(\frac{3}{2}+n\right)+\ln K-A_n-2 A_{n+1}\right)\\
&\chi_2(K)=\frac{12\pi^{3/2}}{K^{1/6}}\left(6-3\ln 12+\ln K\right)+\sum_{n=0}^{\infty}K^{\frac{5}{6}+n}\frac{\Gamma\left(\frac{5}{6}+n\right)\Gamma\left(\frac{7}{6}+n\right)\Gamma\left(\frac{3}{2}+n\right)}{n!\left(n+2\right)!\left(n+2\right)!}\left(-\frac{1}{2}\left(\psi\left(\frac{5}{6}+n\right)+\psi\left(\frac{7}{6}+n\right)+\psi\left(\frac{3}{2}+n\right)+\ln K\right)^2-\frac{1}{2}\psi^{\prime}\left(\frac{5}{6}+n\right)-\frac{1}{2}\psi^{\prime}\left(\frac{7}{6}+n\right)-\frac{1}{2}\psi^{\prime}\left(\frac{3}{2}+n\right)+\left(A_n+2A_{n+1}\left(\right)\right)\left(\psi\left(\frac{5}{6}+n\right)+\psi\left(\frac{7}{6}+n\right)+\psi\left(\frac{3}{2}+n\right)+\ln K\right)-2A_n A_{n+1}-A_{n+1}^2-B_n-2B_{n+1}\right)
\end{align}
And we can obtain the following relations:
\begin{align}
\operatorname{ch}_0=a\chi_0\qquad \operatorname{ch}_1=b\chi_1\qquad \operatorname{ch}_2=c\chi_2-\frac{5}{4}d\chi_0
\end{align}
where $a=\frac{1}{48\sqrt{3}\pi^{3/2}}$, $b=\frac{-i}{48\sqrt{3}\pi^{5/2}}$, $c=\frac{-1}{96\sqrt{3}\pi^{7/2}}$, $d=\frac{1}{48\sqrt{3}\pi^{3/2}}$. Note that the monodromy matrices around $0$ and $1$, which can be refered to T and S transformation respectively, are computed as:
\begin{align}
M_0=\left(
\begin{array}{ccc}
	0 & 1 & 0 \\
	0 & 0 & 1 \\
	-1 & 3 \sqrt[3]{-1} & -3 (-1)^{2/3} \\
\end{array}
\right)
\quad 
M_1=\left(
\begin{array}{ccc}
	-1 & 3 \sqrt[3]{-1} & -3 (-1)^{2/3} \\
	0 & 1 & 0 \\
	0 & 0 & 1 \\
\end{array}
\right)
\end{align}
under the Meilin-Barnes bases \cite{molag:2015monodromy}:
\begin{align}
	I_j(K)=\frac{(-1)^3}{\left(2\pi i\right)^3}\int_L\left(\prod_{i=1}^{3}\Gamma\left(\alpha_i+s\right)\Gamma\left(1-\beta_i-s\right)\right)e^{-3\pi i+2n\pi i}ds
\end{align}
for $j=0,1,2$. In fact we can easily find that:
\begin{align}
&I_0(K)=-\frac{i\left(9\pi^2\chi_0(K)+6i\pi\chi_1(K)+2\chi_2(K)\right)}{8\pi^2}\notag\\
&I_1(K)=-\frac{(-1)^{1/6}\left(\pi^2\chi_0(K)+2i\pi\chi_1(K)+2\chi_2(K)\right)}{8\pi^2}\notag\\
&I_2(K)=\frac{(-1)^{1/3}\left(i\pi^2\chi_0(K)+2\pi\chi_1(K)+2i\chi_2(K)\right)}{8\pi^2}\notag
\end{align}
Therefore we can obtain the monodromy matrix around 0 and 1 under the bases $\operatorname{ch}_0$, $\operatorname{ch}_{1,\log}$, $\operatorname{ch}_{2,\log}$ after suitable conjugation:
\begin{align}
T=M_0^{\prime}=\left(
\begin{array}{ccc}
	-(-1)^{2/3} & 0 & 0 \\
	-2 (-1)^{2/3} & -(-1)^{2/3} & 0 \\
	(-1)^{2/3} & (-1)^{2/3} & -(-1)^{2/3} \\
\end{array}
\right)\qquad
S=M_1^{\prime}=\left(
\begin{array}{ccc}
	0 & 0 & 1 \\
	0 & 1 & 0 \\
	1 & 0 & 0 \\
\end{array}
\right)
\end{align}
